# Supplementary material for: Discrete Probabilistic Inverse Optimal Transport
Source: arXiv:2112.09754 source file (2022-06-21)
Supplement: Supplementary file 1 [file SI_AISTATS_2022.tex]

\documentclass[twoside]{article}

\usepackage{aistats2022}
% If your paper is accepted, change the options for the package
% aistats2022 as follows:
%
%\usepackage[accepted]{aistats2022}
%
% This option will print headings for the title of your paper and
% headings for the authors names, plus a copyright note at the end of
% the first column of the first page.

% If you set papersize explicitly, activate the following three lines:
%\special{papersize = 8.5in, 11in}
%\setlength{\pdfpageheight}{11in}
%\setlength{\pdfpagewidth}{8.5in}

% If you use natbib package, activate the following three lines:
\usepackage[round]{natbib}

% If you use BibTeX in apalike style, activate the following line:
%\bibliographystyle{apalike}

% \usepackage[utf8]{inputenc}
% \usepackage[utf8]{inputenc} % allow utf-8 input
% \usepackage[T1]{fontenc}    % use 8-bit T1 fonts
% \usepackage{hyperref}       % hyperlinks
% \usepackage{url}            % simple URL typesetting
% \usepackage{booktabs}       % professional-quality tables
% \usepackage{amsfonts}       % blackboard math symbols
% \usepackage{nicefrac}       % compact symbols for 1/2, etc.
% \usepackage{microtype}      % microtypography
% \usepackage{fullpage}

\usepackage{graphicx}
\usepackage{color,soul}
\usepackage{amsmath}
\usepackage{amsthm}
\usepackage{amstext}
\usepackage{mathrsfs}
\usepackage{amssymb}
\usepackage{bm}
\usepackage{pictexwd,dcpic}
\usepackage{enumitem}
\usepackage[ruled,vlined]{algorithm2e}
\usepackage{empheq,etoolbox}
% Update display of subequation numbering (Xy) > (X.y)
\usepackage{cases}
\usepackage{cleveref}

\usepackage{tikz}
\usetikzlibrary{calc,intersections,through}
\tikzset{
    partial ellipse/.style args={#1:#2:#3}{
        insert path={+ (#1:#3) arc (#1:#2:#3)}
    }
}

%\usepackage{pgfplots}

%theorem styles

\makeatletter
\newtheorem*{rep@theorem}{\rep@title}
\newcommand{\newreptheorem}[2]{%
\newenvironment{rep#1}[1]{%
\def\rep@title{#2 \ref{##1}}%
\begin{rep@theorem}}%
{\end{rep@theorem}}}
\makeatother

\newtheorem*{thm*}{Theorem}

\newreptheorem{lemma}{Lemma}
\newreptheorem{prop}{Proposition}
\newreptheorem{thm}{Theorem}
\newreptheorem{cor}{Corollary}

\theoremstyle{definition}

\newtheorem*{definition*}{Definition}

\newtheorem*{example*}{Example}

\newtheorem*{framework*}{Unifying OT Framework}

% \theoremstyle{remark}
% \newtheorem{remark}{Remark}

% \newtheorem{theorem}{Theorem}[section]
% \theoremstyle{definition}
% \newtheorem{definition}[theorem]{Definition}
% \newtheorem{proposition}[theorem]{Proposition}
% \newtheorem{example}[theorem]{Example}
% \newtheorem{lemma}[theorem]{Lemma}
% \newtheorem{corollary}[theorem]{Corollary}
% \newtheorem{note}[theorem]{Note}
% \newtheorem{remark}[theorem]{Remark}

% Notations
 % data space
 % hypothesis space
 % all real numbers.
 % a small parameter
%  expectation
%  
%  
%  

% \usepackage[
% backend=biber,
% style=alphabetic,
% sorting=ynt
% ]{biblatex}

%\newcommand{\pat}[1]{\textcolor[rgb]{.7,0,.2}{#1}}

\usepackage[ruled,vlined]{algorithm2e}

\usepackage{xr}
\makeatletter
\newcommand*{\addFileDependency}[1]{% argument=file name and extension
  \typeout{(#1)}
  \@addtofilelist{#1}
  \IfFileExists{#1}{}{\typeout{No file #1.}}
}
\makeatother
 
\newcommand*{\myexternaldocument}[1]{%
    \externaldocument{#1}%
    \addFileDependency{#1.tex}%
    \addFileDependency{#1.aux}%
}

\myexternaldocument{0-AISTATS_2022}

\begin{document}

% If your paper is accepted and the title of your paper is very long,
% the style will print as headings an error message. Use the following
% command to supply a shorter title of your paper so that it can be
% used as headings.
%
%\runningtitle{I use this title instead because the last one was very long}

% If your paper is accepted and the number of authors is large, the
% style will print as headings an error message. Use the following
% command to supply a shorter version of the authors names so that
% they can be used as headings (for example, use only the surnames)
%
%\runningauthor{Surname 1, Surname 2, Surname 3, ...., Surname n}

% Supplementary material: To improve readability, you must use a single-column format for the supplementary material.
\onecolumn
\aistatstitle{Supplementary for Probabilistic Inverse Optimal Transport}
\input{supp_proofs}
\input{supp_algs}

\bibliographystyle{plainnat} 
\bibliography{references}

\end{document}
